# Supplementary material for: A Deep Insight into Measuring Face Image Utility with General and Face-specific Image Quality Metrics
Source: arXiv:2110.11111 source file (2021-10-22)
Supplement: Supplementary file 1 [file 0348_supp.pdf]

## Supplementary Material

### A Deep Insight into Measuring Face Image Utility with General and Face-specific Image Quality Metrics

The Figures and Tables submitted in the supplementary material complement our submitted paper with the title "A Deep Insight into Measuring Face Image Utility with General and Face-specific Image Quality Metrics". The results in the main paper are sufficient to deliver the main messages of the paper. However, we present an extended set of results here to provide a wider and more detailed experimental view for the reviewers.

Figure 1 illustrates the error vs. reject characteristic (ERC) at a fixed false match rate (FMR) of 0.01, namely the FMR1000 for handcrafted image features (solid line, first row), learned image quality assessment (IQA) methods (dashed line, second row) and deep-learning-based (DL-based) face image quality assessment (FIQA) methods (solid line, second row) evaluated on the Biosecure database (DB). These figures go along with Figure 1 and Figure 2 from the main article (for the LFW and VGGFace2 databases). As the image quality of the Biosecure database is too good, no useful trend can be extracted from the ERC plot. Therefore, we only focused on depicting the ERC at FMR1000 for LFW and VGGFace2 databases in the submitted work.

Figure 2 and Figure 3 visualize the ERC at FMR100 (similar plots are shown for FMR1000 in the main article) for handcrafted features (Figure 2), learned IQA methods (dashed line, Figure 3) and DL-based FIQA methods (solid line, Figure 3) evaluated with the Biosecure, LFW, and VGGFace2 database. A similar trend is observed as depicted in Figure 2 from the main article. The inter-eye distance reveals a strong correlation to the face image utility, especially for the uncontrolled VGGFace2. However, the overall performance of the feature-based FIQ is twice as bad as compared to the DL-based FIQA methods. A clear decreasing trend is observed for the IQA methods in the ERC in Figure 3. Even these methods are not superior compared to the DL-based FIQA methods, they still reveal a similar trend to the FIQA methods.

Table 1 completes Table 1 from the main article. The main article only provide the top-3 methods in each category to make an overall comparison across the best-performing methods on LFW database. Here, it depicts the evaluation of all considered all 6 DL-based FIQA, 10 learned IQA, and the 7 feature-based FIQA methods

for the false non-match rate (FNMR) at two reject ratios (20 % and 40 %) based on three FR models (ArcFace, SphereFace, Facenet) respectively. Handcrafted features and other learned IQA methods have similar behaviors, while learned FIQA methods still outperform other methods.

Similarly Table 2 also supplement Table 1 from the main article by listing the results of all methods considered in the main article. The table depicts the evaluation result on the VGGFace2. VGGFace2 is a more general database containing a large variety of uncontrolled face images. DL-based FIQA methods show clear dominance for this database across different settings. The inter-eye distance shows better performance compared to other individual handcrafted features, however is not consistently well-performing across different settings. Therefore, these handcrafted features are less useful as to serve as a generalized and stable metric to relate to face image utility.

Table 3 depicts the evaluation result on the Biosecure database using all methods introduced in the main article. This is an additional table that is not provided in the main article. We shifted it to the supplementary material because the quality of the Biosecure is too good to provide useful insights regarding the research question posed in the main article. As already visible from the ERC plots, no error is made given the correct threshold due to the good quality images provided in the database. Therefore this table makes our analysis complete but does not offer additional useful findings on the posed research question from our main article measuring face image utility with general and face-specific quality metrics.

The matrix is showing the the ratio of overlapped samples between the samples with the lowest/highest 10% qualities as measured by two quality estimation methods (on the X and Y axes). The matrix in Figure 6 and 7 are build on data from LFW, and Figure 4 and 5 are using BioSecure database. These are provided to complete the results from igure 4 in the main article. A large ratio indicates a larger reasoning similarity between the considered pair of methods. As the image quality distribution is quite constrained and controlled for LFW and Biosecure, the results appear more homogeneously. The effectiveness of different methods is more obvious for VGGFace2 in the main article.

**LFW at FMR 1000**

|               |                     | ArcFace |       | Sphereface |       | FaceNet |       |
|---------------|---------------------|---------|-------|------------|-------|---------|-------|
|               |                     | 20%     | 40%   | 20%        | 40%   | 20%     | 40%   |
| DL-based FIQA | PFE                 | 0.697   | 0.478 | 1.444      | 0.878 | 0.747   | 0.478 |
|               | MagFace             | 0.741   | 0.479 | 2.126      | 1.118 | 0.840   | 0.638 |
|               | SDD                 | 0.603   | 0.412 | 2.160      | 1.073 | 0.853   | 0.495 |
|               | FaceQnet            | 0.633   | 0.226 | 2.678      | 1.362 | 1.168   | 0.453 |
|               | rankIQ              | 0.488   | 0.490 | 3.275      | 2.289 | 1.075   | 0.817 |
|               | SER-FIQ(on Arcface) | 0.983   | 0.725 | 3.837      | 2.903 | 2.152   | 1.741 |
| Image Quality | CNNIQA              | 1.015   | 1.048 | 4.264      | 3.930 | 2.385   | 2.183 |
|               | NIQE                | 0.926   | 0.780 | 4.990      | 4.770 | 2.417   | 1.994 |
|               | rankIQA             | 1.178   | 1.158 | 5.072      | 4.189 | 2.715   | 2.584 |
|               | PIQE                | 1.136   | 1.146 | 5.165      | 5.444 | 2.738   | 2.578 |
|               | MEON                | 0.959   | 1.280 | 5.300      | 5.892 | 2.725   | 3.159 |
|               | dipIQ               | 1.159   | 1.049 | 5.331      | 5.228 | 2.921   | 2.887 |
|               | BRISQUE             | 1.082   | 1.113 | 5.361      | 4.795 | 2.835   | 3.253 |
|               | DBCNN               | 1.019   | 0.786 | 5.150      | 4.628 | 2.561   | 2.532 |
|               | DeepIQA             | 1.159   | 1.140 | 5.424      | 5.228 | 2.738   | 3.041 |
|               | UNIQUE              | 1.333   | 1.394 | 6.154      | 6.103 | 2.717   | 2.789 |
| Feature FIQA  | inter eye dist      | 0.902   | 0.831 | 4.914      | 4.492 | 2.658   | 2.747 |
|               | mean                | 0.532   | 0.558 | 3.728      | 3.272 | 1.798   | 1.915 |
|               | sharpness           | 1.248   | 1.355 | 5.794      | 6.271 | 2.797   | 3.220 |
|               | blur                | 0.847   | 0.831 | 4.337      | 3.993 | 2.442   | 1.497 |
|               | contrast            | 0.860   | 0.796 | 4.709      | 4.424 | 2.025   | 1.946 |
|               | sum exposure        | 0.620   | 0.780 | 4.293      | 4.423 | 1.914   | 2.428 |
|               | sym.-intersection   | 1.174   | 1.140 | 5.615      | 4.736 | 2.909   | 2.719 |

| <b>LFW at FMR 100</b> |                     |         |       |            |       |         |       |
|-----------------------|---------------------|---------|-------|------------|-------|---------|-------|
|                       |                     | ArcFace |       | Sphereface |       | FaceNet |       |
|                       |                     | 20%     | 40%   | 20%        | 40%   | 20%     | 40%   |
| DL-based FIQA         | PFE                 | 0.647   | 0.399 | 0.674      | 0.319 | 0.597   | 0.319 |
|                       | MagFace             | 0.692   | 0.479 | 0.790      | 0.559 | 0.642   | 0.559 |
|                       | SDD                 | 0.552   | 0.412 | 0.753      | 0.412 | 0.652   | 0.412 |
|                       | FaceQnet            | 0.584   | 0.226 | 0.681      | 0.226 | 0.584   | 0.151 |
|                       | rankIQ              | 0.439   | 0.408 | 0.684      | 0.572 | 0.488   | 0.408 |
|                       | SER-FIQ(on Arcface) | 0.935   | 0.653 | 1.310      | 1.015 | 1.169   | 0.870 |
| Image Quality         | CNNIQA              | 0.862   | 0.873 | 1.370      | 1.397 | 1.319   | 1.135 |
|                       | NIQE                | 0.720   | 0.433 | 1.388      | 1.127 | 1.234   | 0.867 |
|                       | rankIQA             | 0.973   | 1.158 | 1.434      | 1.426 | 1.178   | 1.336 |
|                       | PIQE                | 0.981   | 0.859 | 1.704      | 1.719 | 1.446   | 1.241 |
|                       | MEON                | 0.858   | 1.110 | 1.665      | 1.793 | 1.362   | 1.622 |
|                       | dipIQ               | 0.973   | 0.962 | 1.435      | 1.224 | 1.383   | 1.399 |
|                       | BRISQUE             | 0.876   | 1.027 | 1.443      | 1.369 | 1.288   | 1.712 |
|                       | DBCNN               | 0.866   | 0.786 | 1.376      | 1.048 | 1.121   | 1.048 |
|                       | DeepIQA             | 1.105   | 1.045 | 1.685      | 1.901 | 1.421   | 1.520 |
|                       | UNIQUE              | 1.128   | 1.307 | 1.794      | 2.005 | 1.435   | 1.569 |
| Feature FIQA          | inter eye dist      | 0.802   | 0.831 | 1.404      | 1.247 | 1.354   | 1.414 |
|                       | mean                | 0.387   | 0.399 | 0.968      | 1.037 | 0.678   | 0.798 |
|                       | sharpness           | 1.049   | 1.271 | 1.648      | 1.864 | 1.448   | 1.610 |
|                       | blur                | 0.697   | 0.748 | 1.246      | 1.164 | 1.146   | 0.998 |
|                       | contrast            | 0.708   | 0.531 | 1.367      | 1.150 | 0.860   | 0.708 |
|                       | sum exposure        | 0.465   | 0.780 | 1.189      | 1.301 | 0.879   | 1.301 |
|                       | sym.-intersection   | 1.020   | 0.964 | 1.786      | 1.578 | 1.480   | 1.228 |

Table 1. The table depicts the evaluation of DL-based FIQA methods, learned IQA methods, and the feature-based FIQA on the LFW DB for the FNMR at two reject ratios (20 % and 40 %) with two setups at FMR1000 and FMR100 based on three FR models (ArcFace, SphereFace, Facenet) respectively. Using the official test protocol from LFW, most methods behave similarly, still one of the FIQA methods dominates the top-1 rank consistently.

**VGGFace2 at FMR 1000**

|               |                     | ArcFace |        | Sphereface |        | FaceNet |        |
|---------------|---------------------|---------|--------|------------|--------|---------|--------|
|               |                     | 20%     | 40%    | 20%        | 40%    | 20%     | 40%    |
| DL-based FIQA | PFE                 | 7.505   | 5.955  | 20.394     | 10.836 | 13.694  | 8.127  |
|               | MagFace             | 7.520   | 6.171  | 21.329     | 11.650 | 13.993  | 8.540  |
|               | SDD                 | 7.508   | 5.931  | 21.836     | 12.371 | 14.905  | 8.987  |
|               | FaceQnet            | 8.494   | 6.875  | 25.864     | 19.211 | 17.441  | 12.721 |
|               | rankIQ              | 9.096   | 8.215  | 25.185     | 19.004 | 18.351  | 14.505 |
|               | SER-FIQ(on Arcface) | 8.703   | 7.137  | 24.466     | 17.279 | 18.421  | 14.167 |
| Image Quality | CNNIQA              | 10.088  | 8.154  | 35.201     | 29.276 | 24.283  | 19.520 |
|               | NIQE                | 12.732  | 13.106 | 41.373     | 41.494 | 29.506  | 29.830 |
|               | rankIQA             | 9.456   | 7.914  | 32.459     | 28.355 | 22.066  | 18.796 |
|               | PIQE                | 9.612   | 9.056  | 35.553     | 34.411 | 23.854  | 22.811 |
|               | MEON                | 9.497   | 7.831  | 32.572     | 29.009 | 22.385  | 19.171 |
|               | dipIQ               | 9.248   | 7.234  | 32.775     | 28.798 | 22.173  | 18.519 |
|               | BRISQUE             | 8.468   | 7.292  | 30.706     | 27.002 | 20.593  | 17.683 |
|               | DBCNN               | 8.565   | 7.246  | 41.815     | 47.275 | 21.012  | 18.144 |
|               | DeepIQA             | 9.587   | 8.157  | 30.813     | 27.502 | 23.038  | 20.117 |
|               | UNIQUE              | 11.385  | 11.138 | 40.141     | 41.220 | 27.655  | 27.810 |
| Feature FIQA  | inter eye dist      | 8.670   | 7.274  | 28.378     | 25.373 | 19.364  | 16.702 |
|               | mean                | 10.611  | 9.796  | 36.088     | 34.573 | 25.628  | 24.578 |
|               | sharpness           | 9.373   | 8.326  | 30.967     | 27.952 | 21.145  | 18.704 |
|               | blur                | 8.774   | 7.152  | 30.966     | 26.590 | 20.773  | 17.460 |
|               | contrast            | 10.866  | 10.508 | 35.724     | 34.117 | 25.098  | 24.235 |
|               | sum exposure        | 11.227  | 10.781 | 37.944     | 37.677 | 26.755  | 26.399 |
|               | sym.-intersection   | 11.309  | 11.036 | 32.646     | 28.836 | 23.624  | 21.906 |

| VGGFace2 at FMR 100 |                     |         |        |            |        |         |        |
|---------------------|---------------------|---------|--------|------------|--------|---------|--------|
|                     |                     | ArcFace |        | Sphereface |        | FaceNet |        |
|                     |                     | 20%     | 40%    | 20%        | 40%    | 20%     | 40%    |
| DL-based FIQA       | PFE                 | 6.393   | 5.104  | 9.763      | 6.130  | 6.950   | 4.897  |
|                     | MagFace             | 6.438   | 5.280  | 10.473     | 6.564  | 7.195   | 5.170  |
|                     | SDD                 | 6.377   | 5.085  | 10.356     | 6.441  | 7.365   | 5.110  |
|                     | FaceQnet            | 6.984   | 5.749  | 12.980     | 8.948  | 8.682   | 6.148  |
|                     | rankIQ              | 7.496   | 6.798  | 13.041     | 10.113 | 9.235   | 7.583  |
|                     | SER-FIQ(on Arcface) | 7.274   | 6.113  | 13.120     | 9.581  | 9.461   | 7.404  |
| Image Quality       | CNNIQA              | 8.157   | 6.712  | 19.511     | 15.466 | 12.755  | 9.742  |
|                     | NIQE                | 10.216  | 10.504 | 23.585     | 23.951 | 16.243  | 16.638 |
|                     | rankIQA             | 7.743   | 6.592  | 17.551     | 14.522 | 11.452  | 9.149  |
|                     | PIQE                | 7.747   | 7.245  | 18.965     | 18.206 | 12.095  | 11.509 |
|                     | MEON                | 7.702   | 6.396  | 17.713     | 14.974 | 11.348  | 9.159  |
|                     | dipIQ               | 7.578   | 5.940  | 17.597     | 14.405 | 11.260  | 8.702  |
|                     | BRISQUE             | 6.939   | 6.025  | 16.058     | 13.574 | 10.124  | 8.386  |
|                     | DBCNN               | 7.028   | 6.002  | 16.390     | 14.268 | 10.784  | 8.851  |
|                     | DeepIQA             | 7.805   | 6.633  | 18.067     | 15.579 | 11.789  | 9.918  |
|                     | UNIQUE              | 9.086   | 8.949  | 22.409     | 22.897 | 14.762  | 14.861 |
| Feature FIQA        | inter eye dist      | 7.175   | 6.115  | 14.447     | 12.261 | 9.410   | 7.762  |
|                     | mean                | 8.435   | 7.710  | 20.242     | 19.110 | 13.760  | 13.298 |
|                     | sharpness           | 7.586   | 6.827  | 16.150     | 14.210 | 10.553  | 9.047  |
|                     | blur                | 7.218   | 5.910  | 16.356     | 13.531 | 10.524  | 8.413  |
|                     | contrast            | 8.714   | 8.389  | 20.150     | 19.445 | 13.586  | 13.179 |
|                     | sum exposure        | 8.922   | 8.536  | 21.298     | 21.032 | 14.407  | 14.135 |
|                     | sym.-intersection   | 9.145   | 9.050  | 18.003     | 16.261 | 12.335  | 11.551 |

Table 2. The table depicts the evaluation of DL-based FIQA methods, learned IQA methods, and the feature-based FIQA on the VGGFace2 for the FNMR at two reject ratios (20 % and 40 %) with two setups at FMR1000 and FMR100 based on three FR models (ArcFace, SphereFace, Facenet) respectively.

| BioSecure at FMR 1000 |                     |         |       |            |       |         |       |
|-----------------------|---------------------|---------|-------|------------|-------|---------|-------|
|                       |                     | ArcFace |       | Sphereface |       | FaceNet |       |
|                       |                     | 20%     | 40%   | 20%        | 40%   | 20%     | 40%   |
| DL-based FIQA         | PFE                 | 0.000   | 0.000 | 0.000      | 0.000 | 0.024   | 0.031 |
|                       | MagFace             | 0.000   | 0.000 | 0.000      | 0.000 | 0.035   | 0.011 |
|                       | SDD                 | 0.000   | 0.000 | 0.000      | 0.000 | 0.018   | 0.012 |
|                       | FaceQnet            | 0.000   | 0.000 | 0.030      | 0.000 | 0.000   | 0.000 |
|                       | rankIQ              | 0.000   | 0.000 | 0.019      | 0.030 | 0.000   | 0.000 |
|                       | SER-FIQ(on Arcface) | 0.000   | 0.000 | 0.029      | 0.000 | 0.009   | 0.000 |
| Image Quality         | CNNIQA              | 0.000   | 0.000 | 0.021      | 0.035 | 0.031   | 0.035 |
|                       | NIQE                | 0.000   | 0.000 | 0.033      | 0.019 | 0.000   | 0.000 |
|                       | rankIQA             | 0.000   | 0.000 | 0.056      | 0.020 | 0.011   | 0.000 |
|                       | PIQE                | 0.000   | 0.000 | 0.011      | 0.000 | 0.000   | 0.000 |
|                       | MEON                | 0.000   | 0.000 | 0.033      | 0.020 | 0.000   | 0.000 |
|                       | dipIQ               | 0.000   | 0.000 | 0.032      | 0.018 | 0.021   | 0.036 |
|                       | BRISQUE             | 0.000   | 0.000 | 0.020      | 0.016 | 0.040   | 0.000 |
|                       | DBCNN               | 0.000   | 0.000 | 0.065      | 0.099 | 0.037   | 0.024 |
|                       | DeepIQA             | 0.000   | 0.000 | 0.043      | 0.043 | 0.028   | 0.028 |
|                       | UNIQUE              | 0.000   | 0.000 | 0.046      | 0.025 | 0.038   | 0.064 |
| Feature FIQA          | inter eye dist      | 0.000   | 0.000 | 0.033      | 0.019 | 0.000   | 0.000 |
|                       | mean                | 0.000   | 0.000 | 0.043      | 0.000 | 0.000   | 0.000 |
|                       | sharpness           | 0.000   | 0.000 | 0.032      | 0.051 | 0.000   | 0.000 |
|                       | blur                | 0.000   | 0.000 | 0.055      | 0.020 | 0.33    | 0.000 |
|                       | contrast            | 0.000   | 0.000 | 0.042      | 0.017 | 0.010   | 0.000 |
|                       | sum exposure        | 0.000   | 0.000 | 0.020      | 0.016 | 0.000   | 0.000 |
|                       | sym.-intersection   | 0.000   | 0.000 | 0.053      | 0.070 | 0.042   | 0.070 |

| BioSecure at FMR 100 |                     |         |     |            |     |         |     |
|----------------------|---------------------|---------|-----|------------|-----|---------|-----|
|                      |                     | ArcFace |     | Sphereface |     | FaceNet |     |
|                      |                     | 20%     | 40% | 20%        | 40% | 20%     | 40% |
| DL-based FIQA        | PFE                 | 0       | 0   | 0          | 0   | 0       | 0   |
|                      | MagFace             | 0       | 0   | 0          | 0   | 0       | 0   |
|                      | SDD                 | 0       | 0   | 0          | 0   | 0       | 0   |
|                      | FaceQnet            | 0       | 0   | 0          | 0   | 0       | 0   |
|                      | rankIQ              | 0       | 0   | 0          | 0   | 0       | 0   |
|                      | SER-FIQ(on Arcface) | 0       | 0   | 0          | 0   | 0       | 0   |
| Image Quality        | CNNIQA              | 0       | 0   | 0          | 0   | 0       | 0   |
|                      | NIQE                | 0       | 0   | 0          | 0   | 0       | 0   |
|                      | rankIQA             | 0       | 0   | 0          | 0   | 0       | 0   |
|                      | PIQE                | 0       | 0   | 0          | 0   | 0       | 0   |
|                      | MEON                | 0       | 0   | 0          | 0   | 0       | 0   |
|                      | dipIQ               | 0       | 0   | 0          | 0   | 0       | 0   |
|                      | BRISQUE             | 0       | 0   | 0          | 0   | 0       | 0   |
|                      | DBCNN               | 0       | 0   | 0          | 0   | 0       | 0   |
|                      | DeepIQA             | 0       | 0   | 0          | 0   | 0       | 0   |
|                      | UNIQUE              | 0       | 0   | 0          | 0   | 0       | 0   |
| Feature FIQA         | inter eye dist      | 0       | 0   | 0          | 0   | 0       | 0   |
|                      | mean                | 0       | 0   | 0          | 0   | 0       | 0   |
|                      | sharpness           | 0       | 0   | 0          | 0   | 0       | 0   |
|                      | blur                | 0       | 0   | 0          | 0   | 0       | 0   |
|                      | contrast            | 0       | 0   | 0          | 0   | 0       | 0   |
|                      | sum exposure        | 0       | 0   | 0          | 0   | 0       | 0   |
|                      | sym.-intersection   | 0       | 0   | 0          | 0   | 0       | 0   |

Table 3. The table depicts the evaluation of DL-based FIQA methods, learned IQA methods, and the feature-based FIQA on the BioSecure DB for the FNMR at two reject ratios (20 % and 40 %) with two setups at FMR1000 and FMR100 based on three FR models (ArcFace, SphereFace, Facenet) respectively.

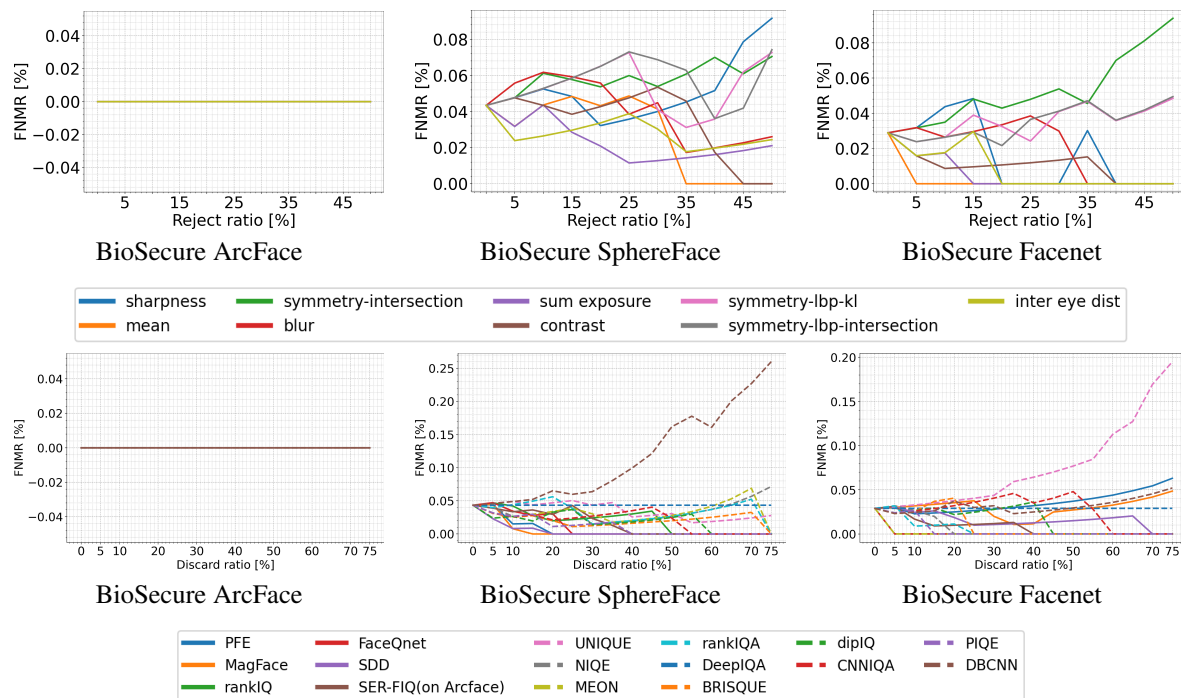

Figure 1. The curves show error vs. reject characteristics at FMR1000 (first three figures) and FMR100 (last three figures) on handcrafted features, learned IQA methods, and DL-based FIQA methods. The rows reveal the ERC results for different face embeddings on BioSecure database. Because the image quality of the Biosecure database is consistently well controlled, no useful trend can be extracted from the ERC plot.

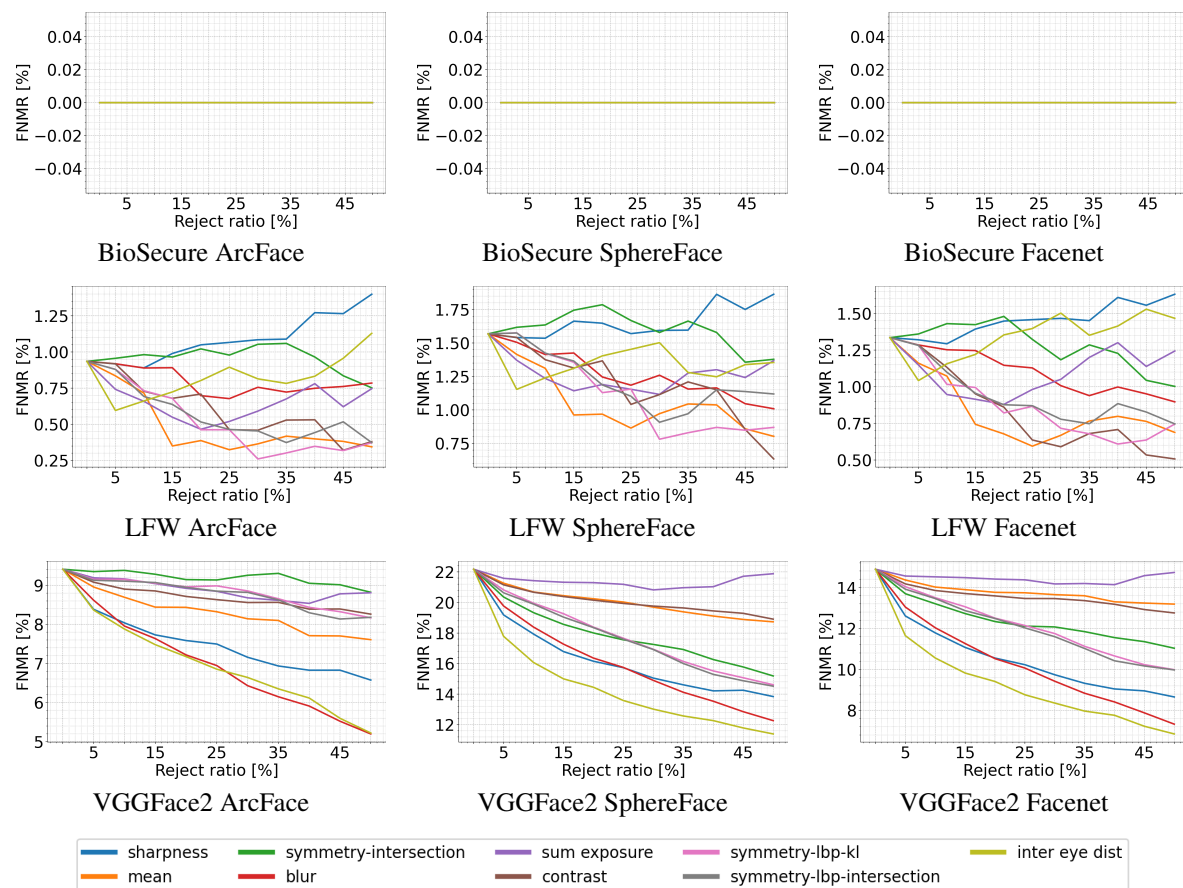

Figure 2. The curves show error vs. reject characteristics at FMR100 on handcrafted features of face images. The rows show the ERC results for different face embeddings on BioSecure, LFW, and VGGFace2. Inter-eye distance performed well on VGGFace2 using original images, while sharpness and blur are well performed for aligned images. However, individual feature contributes inconsistently across different settings as the case for FMR1000.

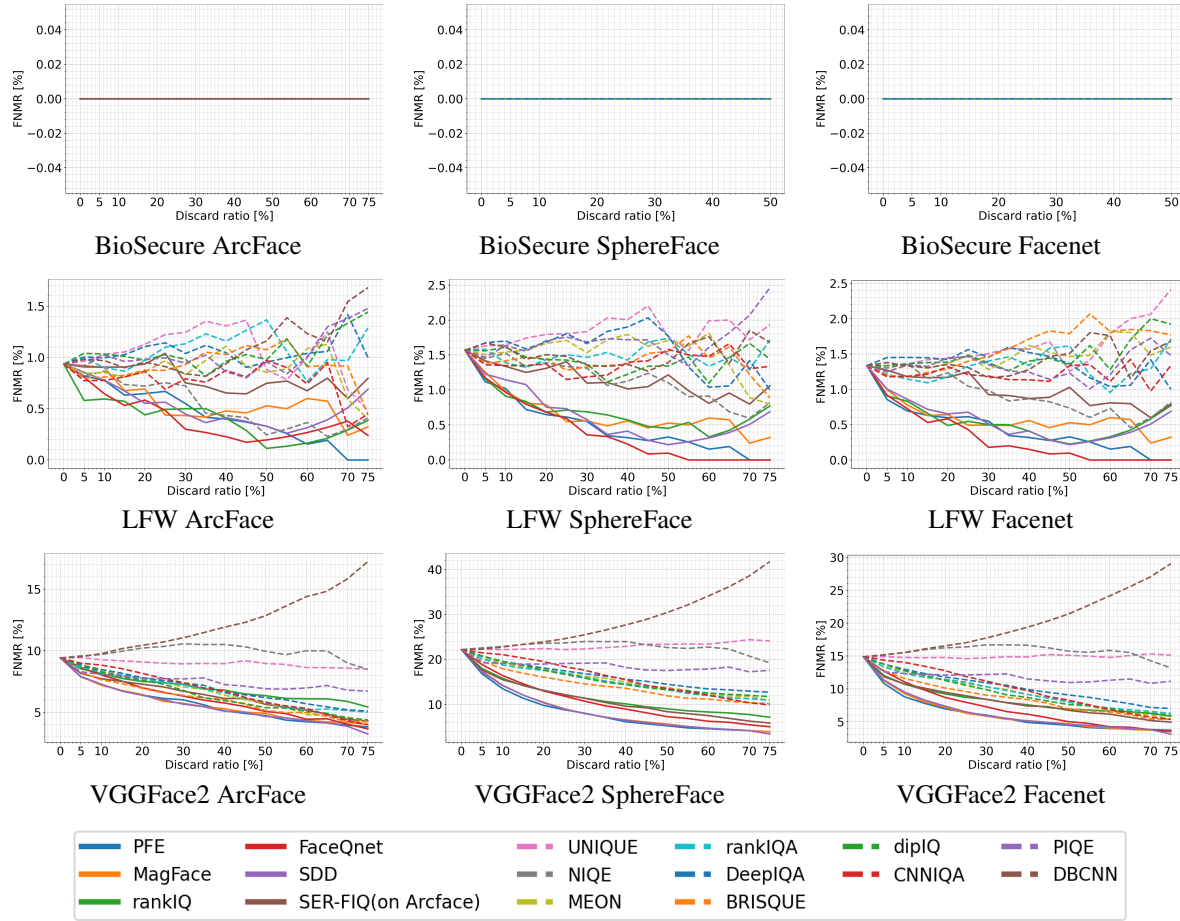

Figure 3. Performance for the predicted face utility based on IQA (dashed lines) and DL-based FIQA (solid lines) methods is shown. The curves show ERCs at FMR100. The rows show the results for diverse face embeddings on BioSecure, LFW, and VGGFace2. DL-based FIQA methods outperform IQA methods on most of the setups. The correlation between learned IQA methods and the face image utility remains observable in this experiment with a decreasing trend in the error rate.

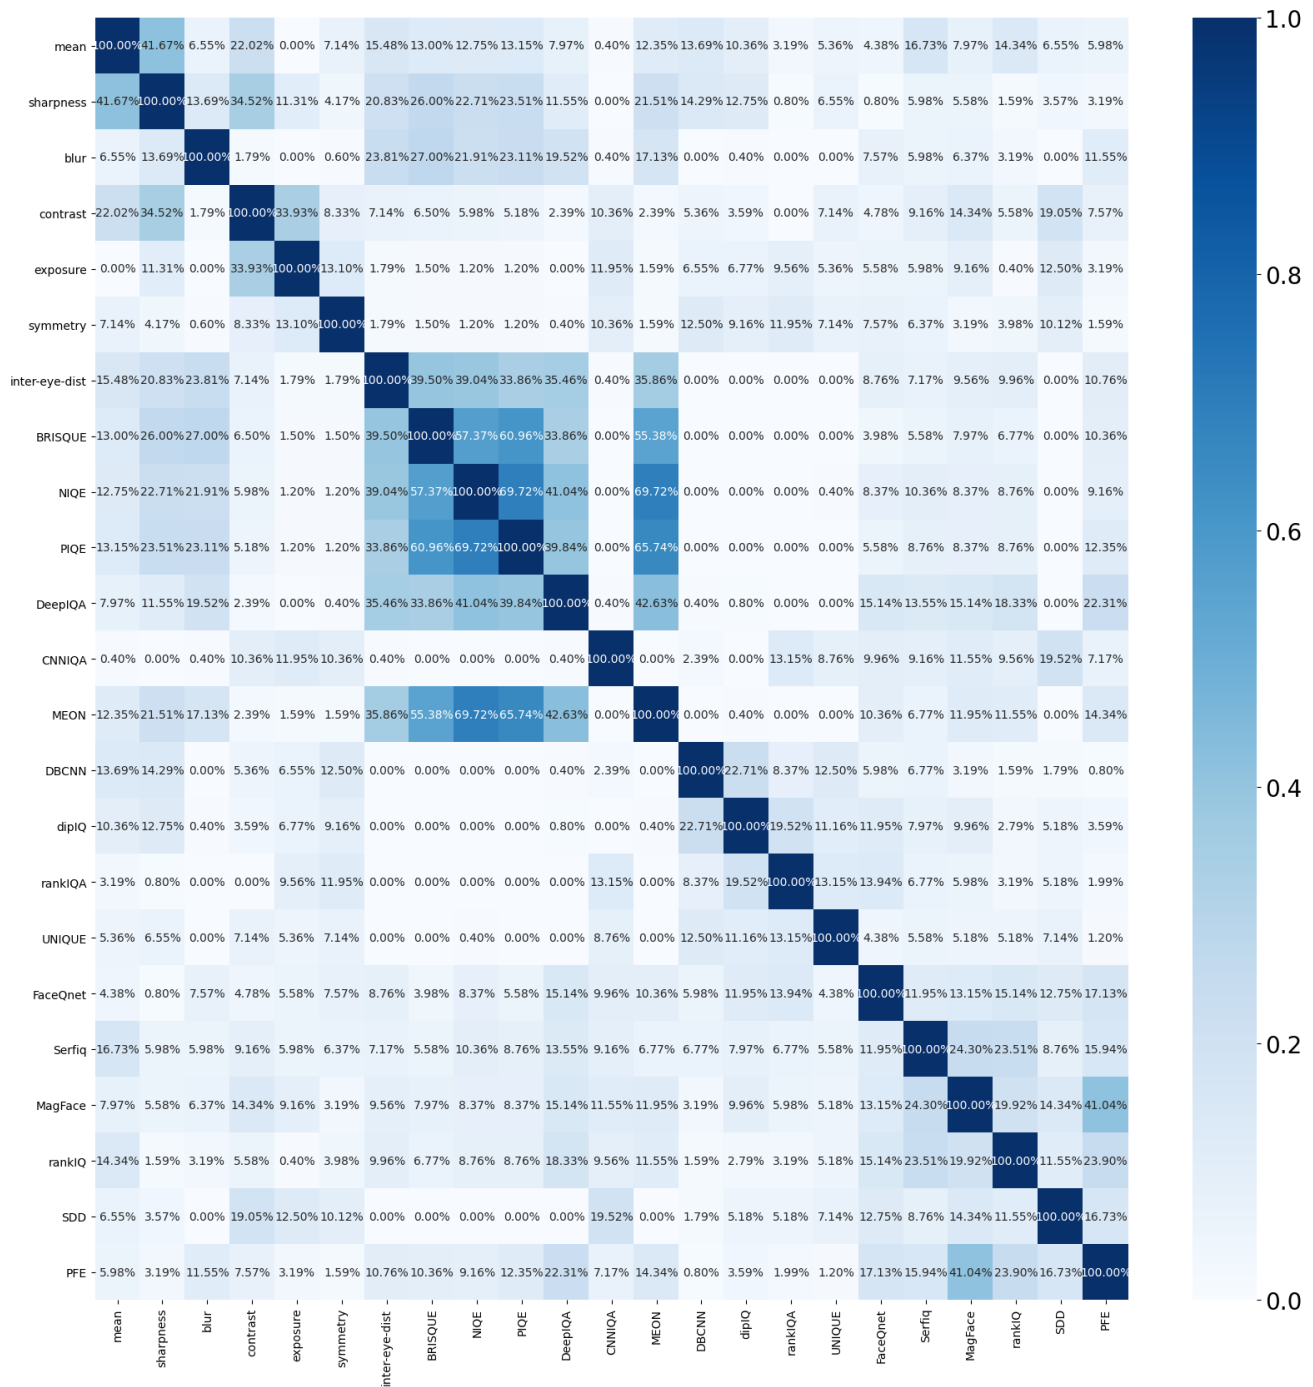

Figure 4. The confusion matrix shows the ratio of overlapped samples between the samples with the lowest 10% qualities (lowest on the left matrix and highest on the right matrix) as measured by two quality estimation methods (on the X and Y axes). The data are extracted from BioSecure database.

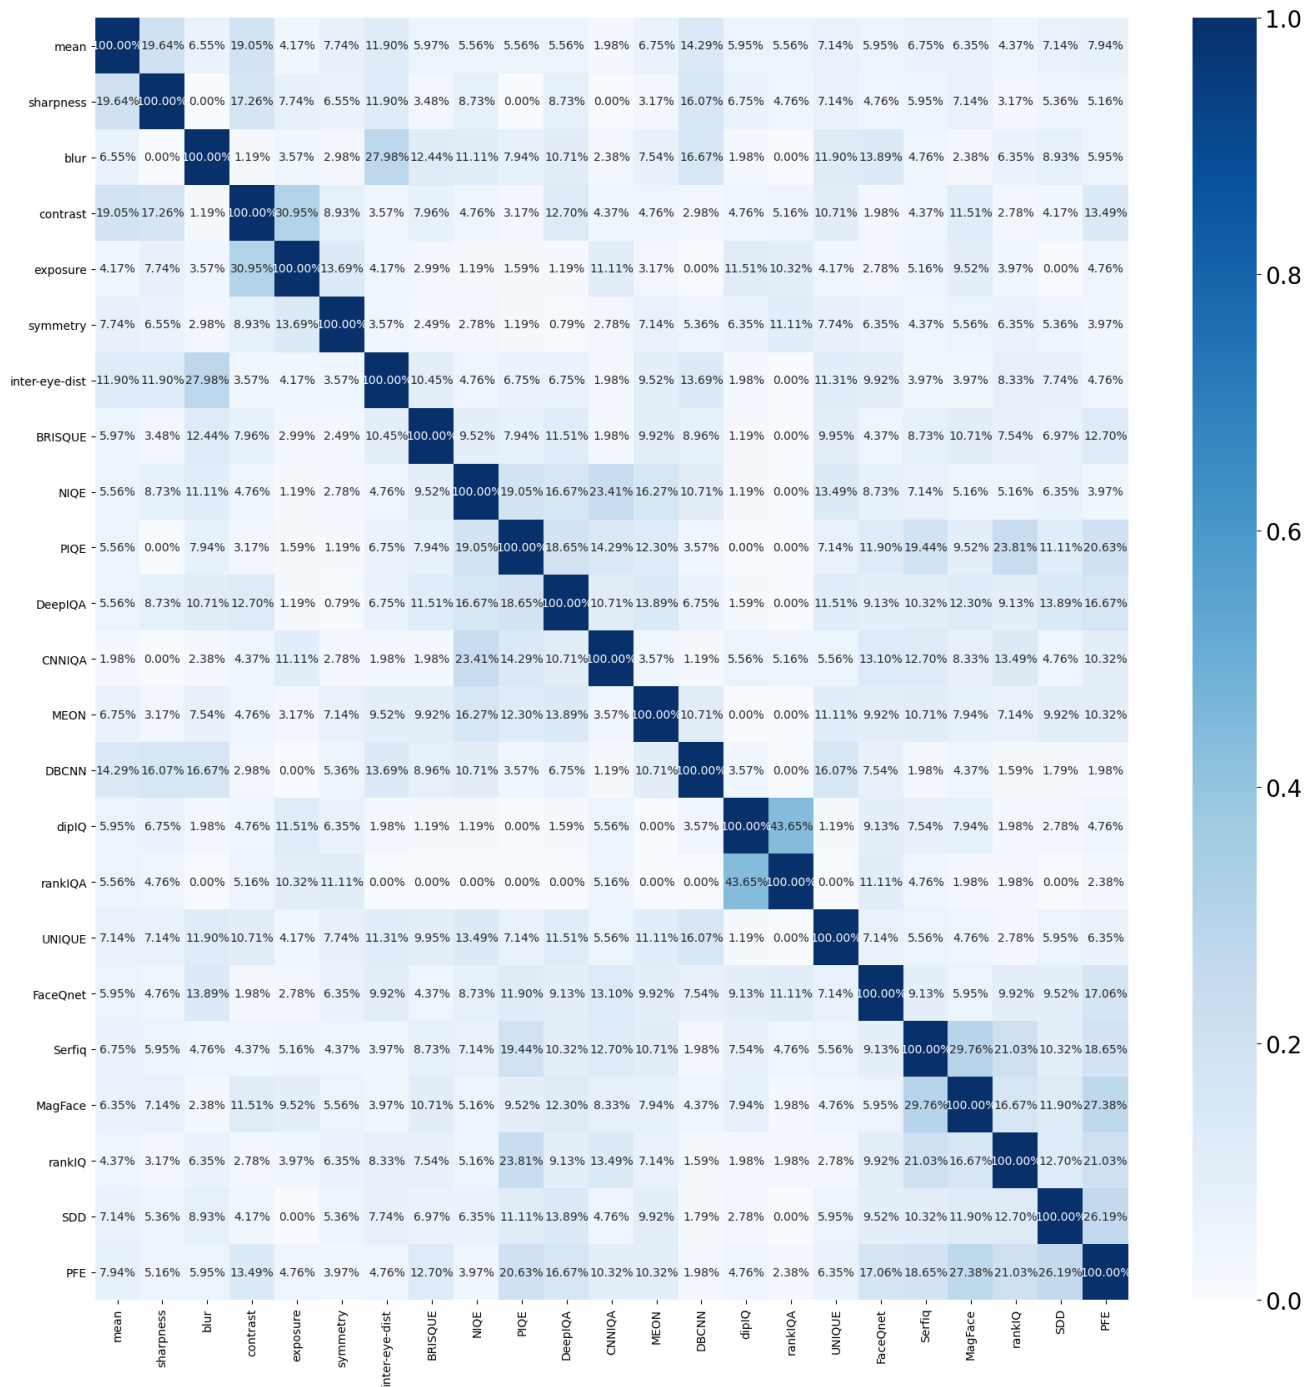

Figure 5. The confusion matrix shows the ratio of overlapped samples between the samples with the highest 10% qualities (lowest on the left matrix and highest on the right matrix) as measured by two quality estimation methods (on the X and Y axes). The data are extracted from BioSecure database.

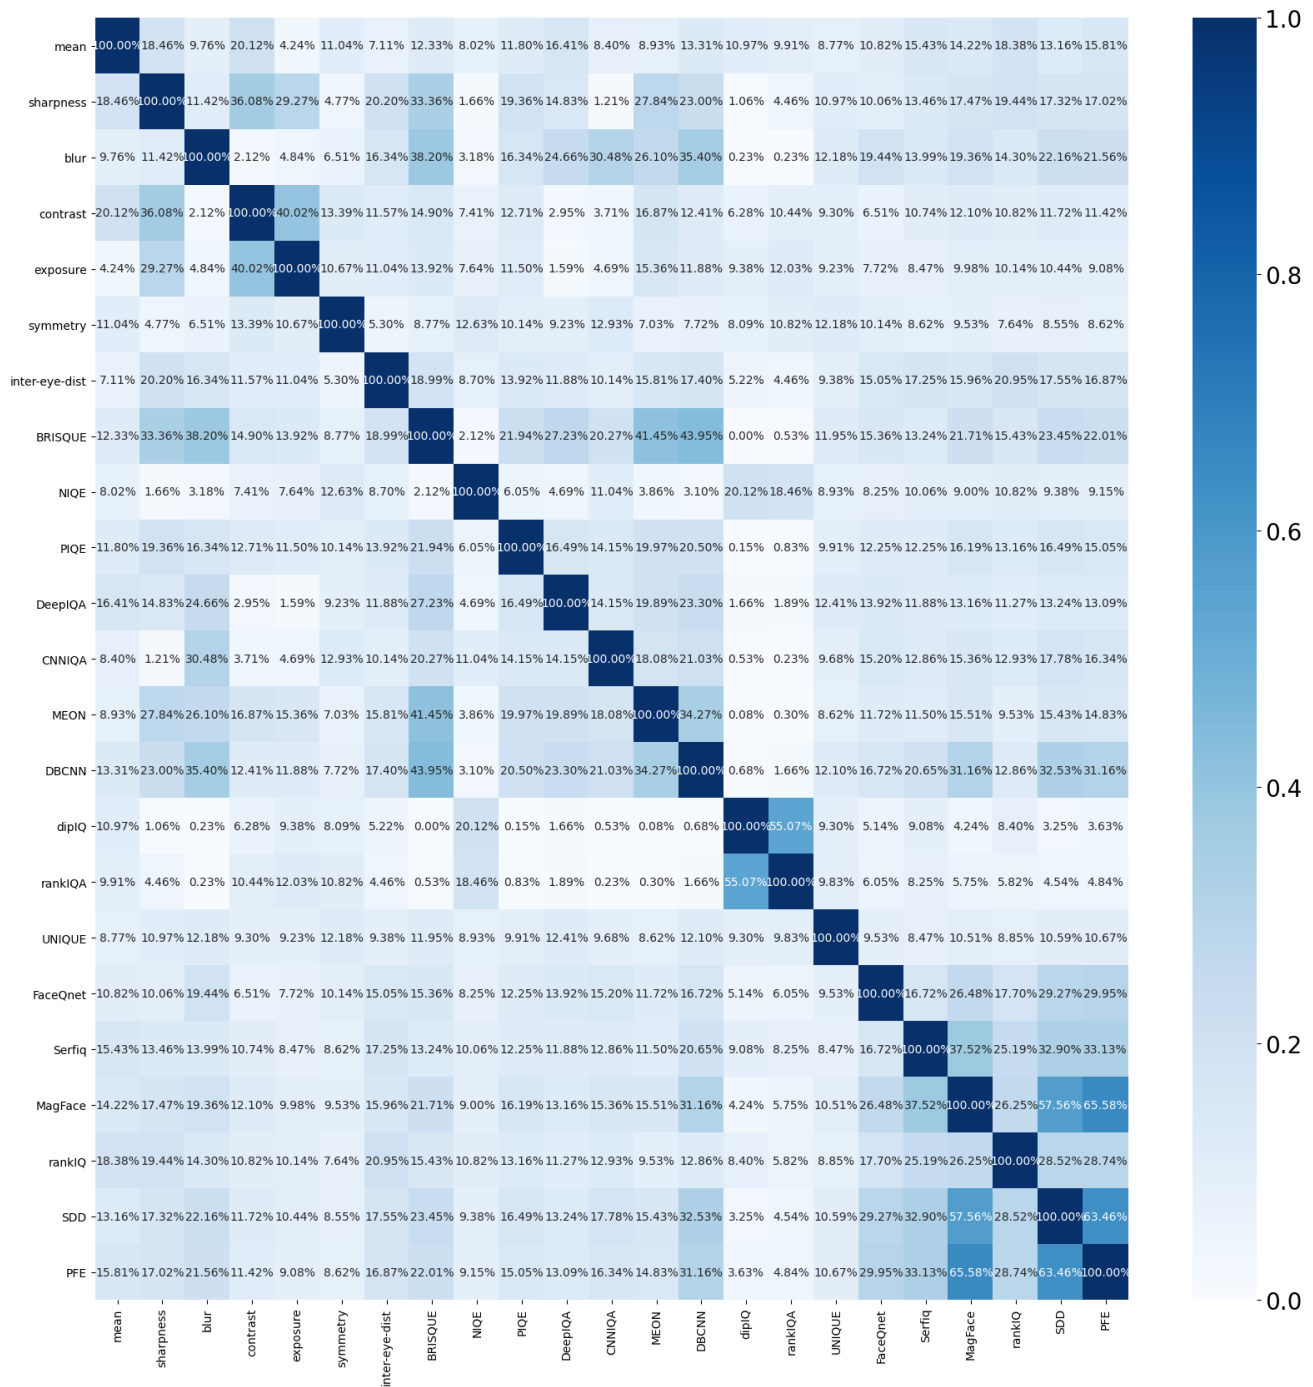

Figure 6. The confusion matrix shows the ratio of overlapped samples between the samples with the lowest 10% qualities (lowest on the left matrix and highest on the right matrix) as measured by two quality estimation methods (on the X and Y axes). The data are extracted from LFW database.

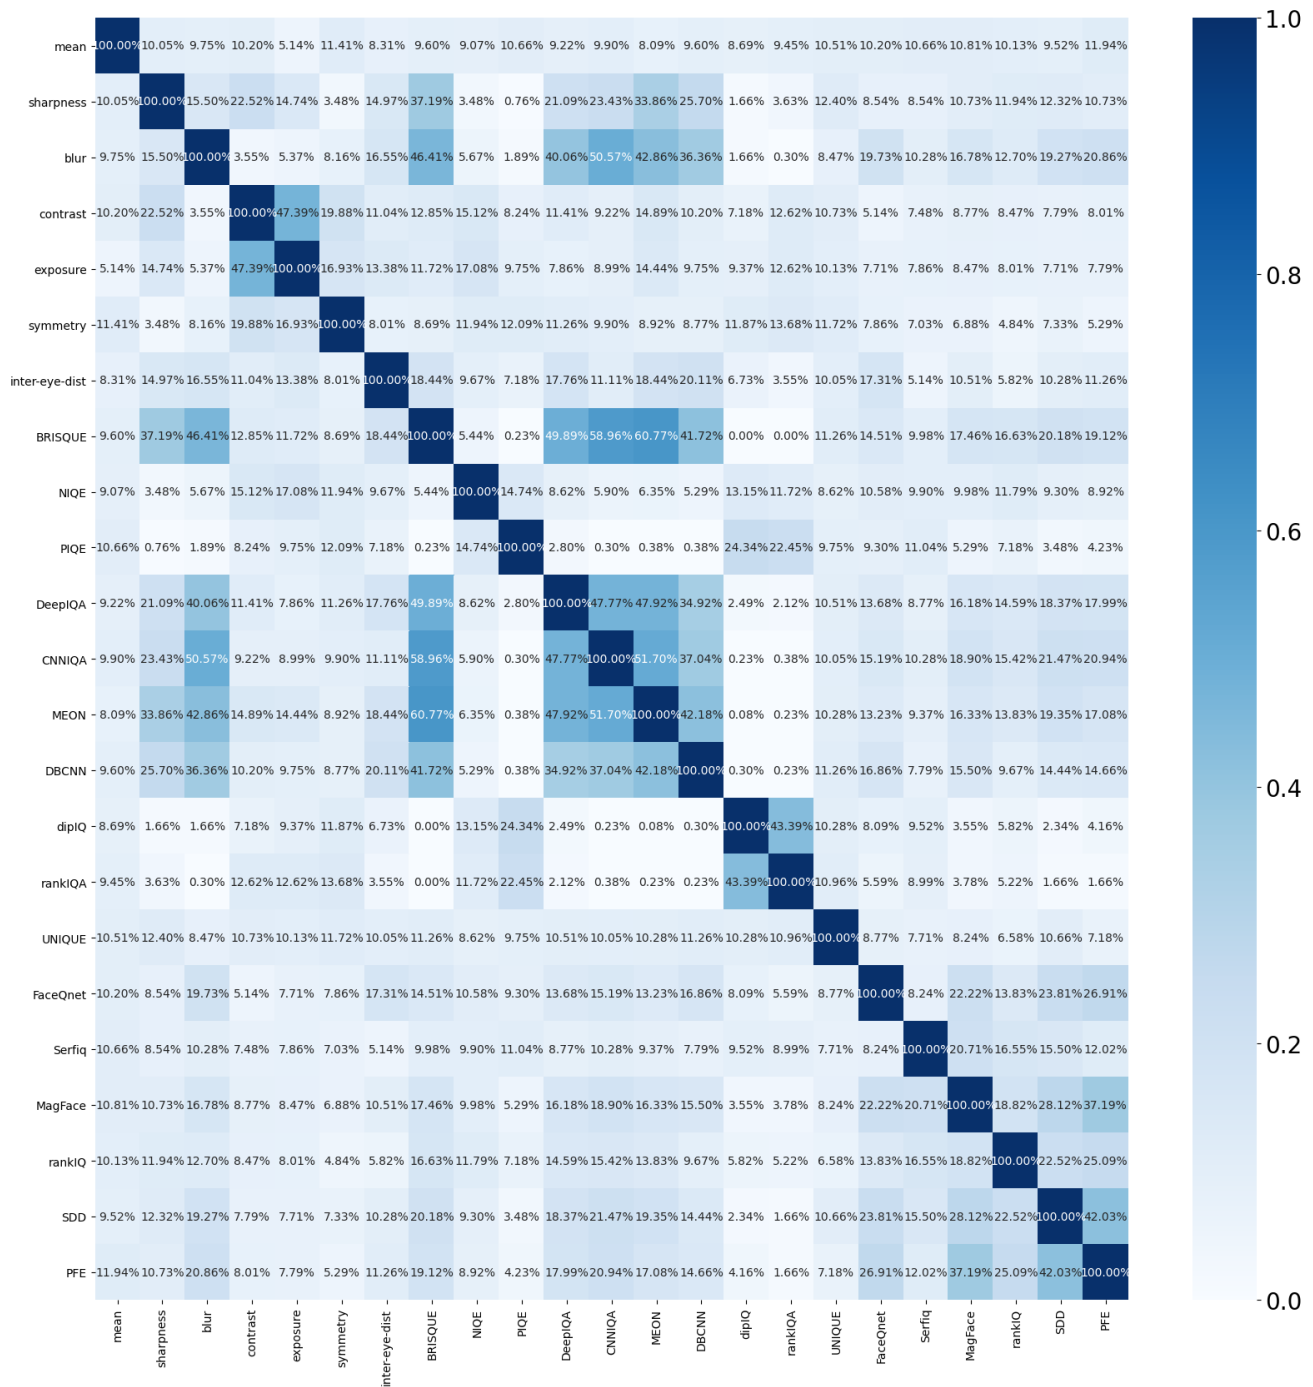

Figure 7. The confusion matrix shows the ratio of overlapped samples between the samples with the highest 10% qualities (lowest on the left matrix and highest on the right matrix) as measured by two quality estimation methods (on the X and Y axes). The data are extracted from LFW database.
